# Supplementary material for: Tuning non-collinear magnetic states by hydrogenation
Source: arXiv:1812.07016 ancillary file (2018-12-17)
Supplement: Supplementary file 1 [file supplement.pdf]

# Tuning non-collinear magnetic states by hydrogenation
## Supplementary Information

Aurore Finco, Pin-Jui Hsu, Kirsten von Bergmann, and Roland Wiesendanger

*Department of Physics, University of Hamburg, D-20355 Hamburg, Germany*

## S1 Hollow state in the hexagonal phase

As mentioned in the main text, there are two possible highly symmetric options for the magnetic configuration of the hexagonal nanoskyrmion lattice in the hexagonal phase of the hydrogenated Fe monolayer on Ir(111). The point where the out-of-plane component of the magnetic moment is maximal can be located either on a top site of the Fe lattice (on-top state) or in a hollow site (hollow state). The SP-STM simulations shown in the main text correspond to the on-top state. However, the results are very similar for the hollow state, as shown in the figures S1, S2 and S3. Note that for the hollow state, there are two possibilities, the site with maximal out-of-plane moment can be either fcc or hcp. Only one of them is depicted here. Our measurements do not allow to distinguish between the on-top and the hollow state concerning the hexagonal nanoskyrmion lattice in the $p2 \times 2)$ H superstructure. In the case of the hexagonal nanoskyrmion lattice in the pristine hcp Fe monolayer, it was possible to conclude that the hollow state is the actual magnetic state [1] based on measurements of the tunneling anisotropic magnetoresistance (TAMR) [2]. In the present case, no TAMR signal could be observed. The reason for this might be that the TAMR contrast is very small and hidden by the structural contrast arising from the H superstructure. Further theoretical studies are thus necessary in order to decide which state (on-top or hollow) is realized in the sample.

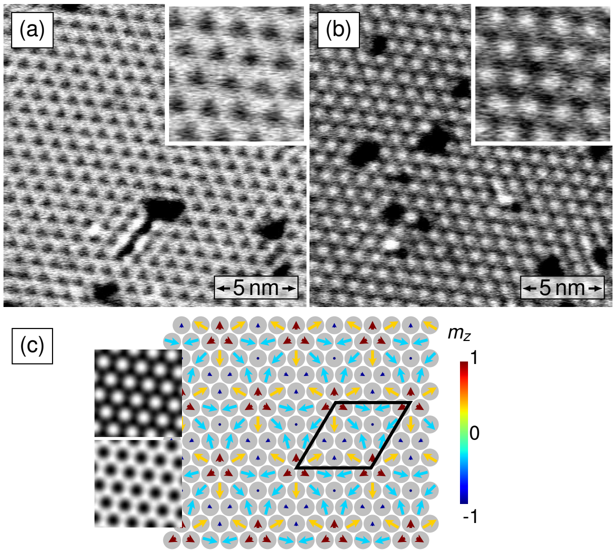


Figure S1: **Hollow state configuration of the hexagonal nanoskyrmion lattice.** (a)-(b) Differential conductance maps showing the oppposite magnetic domains in the hexagonal phase of the hydrogenated Fe monolayer on Ir(111). The insets show magnified views of the data. Measurement parameters: $-1$ V, 1 nA, 4 K, Cr bulk tip. (c) Representation of the hollow state configuration of the hexagonal nanoskyrmion lattice. In this configuration, the points where the out-of-plane component of the magnetization is maximal are located in hollow sites of the atomic lattice. The insets show SP-STM simulation of the two magnetic domains, displayed with the same lateral scale as the data in (a)-(b). The SP-STM simulations were performed with the following realistic parameters: tip-sample distance: 600 pm, work function: 4.8 eV, spin polarization of sample (s) and tip (t): $P_sP_t = 0.2$.

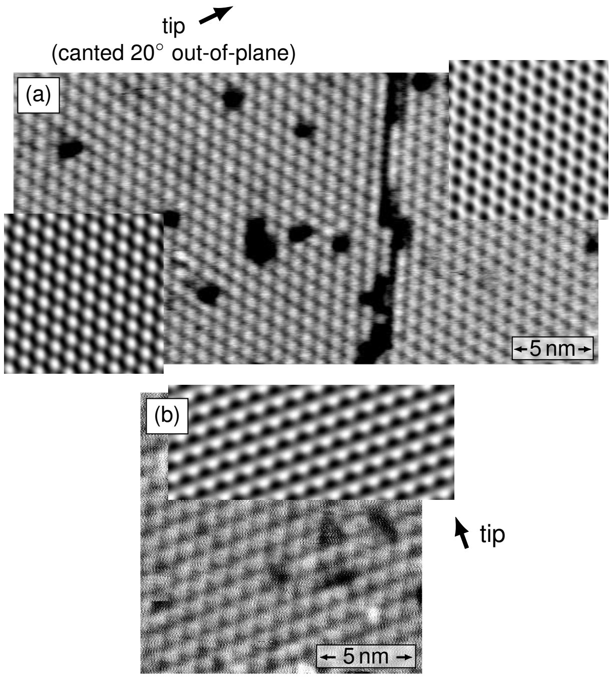


Figure S2: **In-plane components of the hollow state.** (a) Spin-resolved differential conductance map showing the two magnetic domains. The dark line coincides with the boundary between the magnetic domains. The image was measured with a tip sensitive slightly to the out-of-plane and mostly to the in-plane component of the sample magnetization indicated by the arrow. The corresponding SP-STM simulations of the hollow state for both domains are shown in the insets. (b) Spin-resolved differential conductance map showing another in-plane component of the magnetic state and the corresponding SP-STM simulation of the hollow state as inset. Measurement parameters: (a): $-700$ mV, 1 nA, 4 K, 0 T, Cr bulk tip, (b): $-1$ V, 1 nA, 8 K, 0 T, Fe coated W tip. The SP-STM simulations were performed with the following realistic parameters: tip-sample distance: 600 pm, work function: 4.8 eV, spin polarization of sample (s) and tip (t): $P_s P_t = 0.2$.

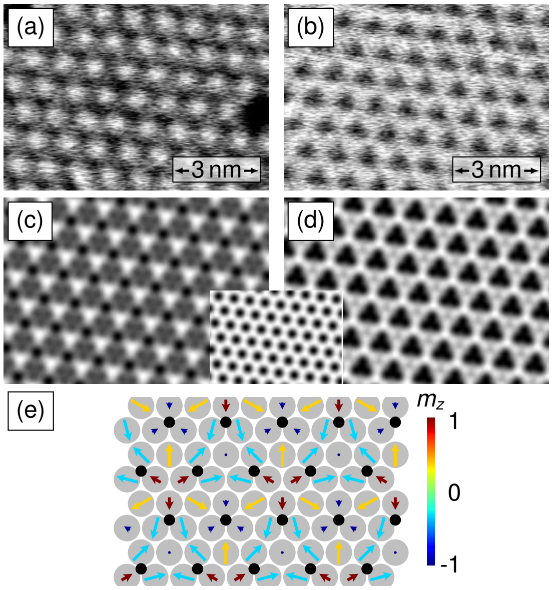


Figure S3: **Position of the H atoms in the hollow state.** (a)-(b) Spin-resolved differential conductance map showing the magnetic state in the hexagonal phase, measured with an out-of-plane sensitive magnetic tip. The images (a) and (b) show the two opposite magnetic domains. Small darker dots are visible between the bright dots in image (a) and the dark dots in image (b) have a triangular shape. These features appear because the position of the H atoms are also visible in addition to the magnetic pattern. Measurement parameters: $-1$ V, 1 nA, 4 K. (c)-(d) SP-STM simulations of the hollow state for an out-of-plane sensitive tip with an additional modulation reproducing the effect of the H atoms and allowing to reproduce the experimental data. The inset shows the pattern used to simulate the contribution of the H atoms. (e) Spin configuration of the hollow state showing the position of the H atoms which allows to reproduce the experimental data. The SP-STM simulations were performed with the following realistic parameters: tip-sample distance: 600 pm, work function: 4.8 eV, spin polarization of sample (s) and tip (t): $P_sP_t = 0.2$.

# S2 Position of the H atoms with respect to the magnetic unit cell in the hexagonal phase

There are eight different possibilities to choose the positions of the H atoms in the $p(2 \times 2)$ superstructure (see sketch in Fig. 2(b) of the main text) with respect to the magnetic unit cell. These configurations are displayed in the sketch at the top of figure S4 with different colors. There are four H atoms per magnetic unit cell, represented for each possibility by 4 dots of the same color. The boundaries of the magnetic unit cell are indicated with the black line. The corners of the displayed unit cell correspond to the points where the out-of-plane magnetic moment is maximum for the on-top and the hollow state.

In order to check if the features observed in the experiment can be understood by the presence of an additional contrast induced by the H atoms, we added a pattern of dark dots with the period of the $p(2 \times 2)$ superstructure to the SP-STM simulations of the two opposite magnetic domains for the on-top and the hollow state, assuming a tip with out-of-plane magnetization. The resulting images are shown in figure S4. Most of the obtained configurations break the three-fold symmetry and are thus not compatible with the experiments performed with out-of-plane sensitive magnetic tips. However, the positions 2 and 7 reproduce the pattern found in the experiment in the case of the on-top state. These two configurations are equivalent, the difference between them is only a $180^\circ$ rotation. A similar result is obtained for the hollow state when the H atoms are at the position 1. Here the $180^\circ$ rotation is not a symmetry of the system and thus only one position of the H atoms allows to generate the observed pattern.

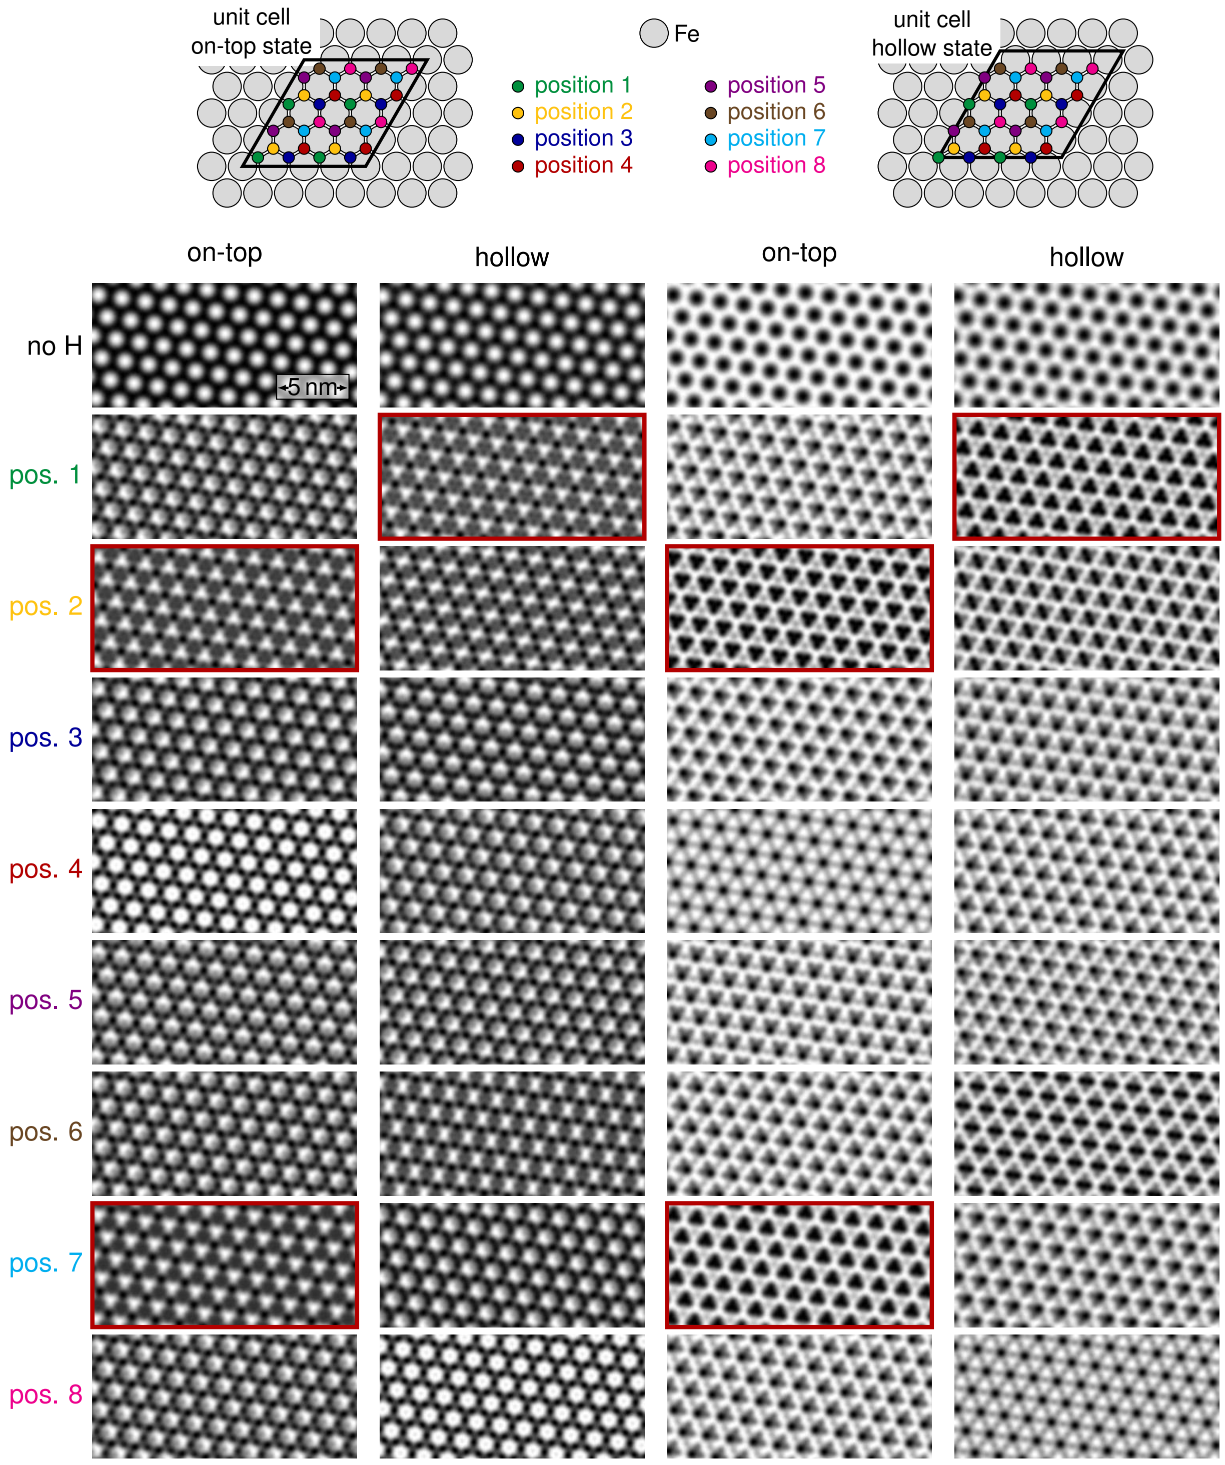


Figure S4: **Investigation of the position of the H atoms in the hexagonal phase.** Full set of SP-STM simulations taking into account the presence of H atoms for the on-top and the hollow spin configurations, considering the 8 possible positions of the H atoms within the magnetic unit cell as indicated by the sketches. The images which agree with the experimental data are marked in red. The SP-STM simulations were performed with the following realistic parameters: tip-sample distance 600 pm, work function 4.8 eV, spin polarization of sample (s) and tip (t): $P_s P_t = 0.2$.

# S3 Excluded magnetic configurations for the roughly square phase

The model for the magnetic state of the roughly square phase presented in figure 6 of the main text corresponds to the superposition of two cycloidal spin spirals with wave vectors chosen to obtain the magnetic cell found in the experimental data. The magnetic moments are normalized after the superposition to keep them constant. The phase shift between the spirals and their position with respect to the atomic lattice were chosen for symmetry reasons. The options which have not been selected are depicted in figure S5.

In the model (a), the corners of the magnetic unit cell (the points where the out-of-plane magnetic moment is maximal) are located in bridge sites of the atomic lattice. In this case, the magnetic structure does not have a mirror symmetry i.e. it should occur not only in three rotational domains but in total six different domains should occur. This is the reason why the model shown in the main text was preferred. In the model (b), the corners of the magnetic unit cell are in the hollow sites. This model was excluded because the out-of-plane magnetic moment is not compensated within each unit cell: the center of the unit cell, where the opposite out-of-plane magnetization is expected, is positioned on a different site of the atomic lattice. Since the experiments do not show the existence of two opposite magnetic domains and since an external magnetic field of 9 T does not induce any change, this model does not agree with the experiment. Finally, in the model (c) the corners of the magnetic unit cell are located on top sites. In this case, some of the magnetic moments are not defined because they vanish in the superposition of the two spirals. Furthermore, the center and the corners of the unit cell are again not equivalent with respect to the Fe atoms. Therefore we preferred the model shown in the main text, in which this is the case.

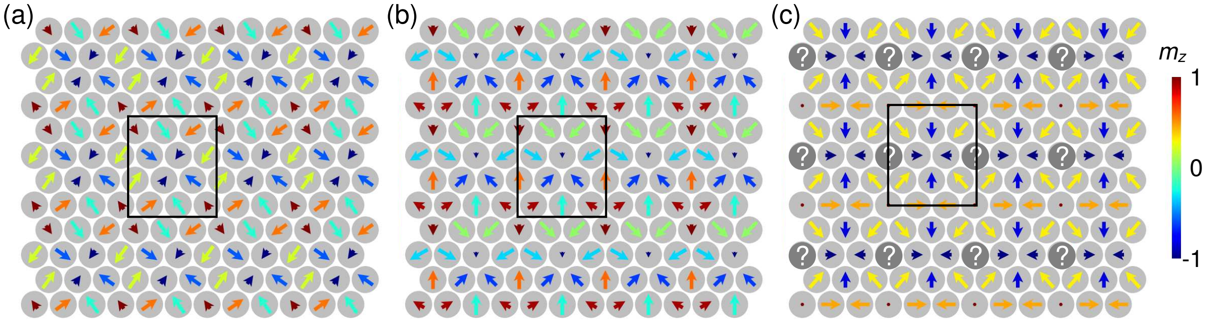


Figure S5: **Choice of the spin configuration model for the square phase.** Representation of other magnetic states exhibiting the magnetic unit cell corresponding to the experimental data for the square phase. They are obtained by shifting on the atomic lattice the spirals used to build the model shown in the main text. In the state (a), the point where the magnetic moment is pointing up is located on a bridge site, and the structure does not have a mirror symmetry. In configuration (b), this point is located on a hollow site and the out-of-plane magnetic moment is not compensated within the unit cell. In configuration (c), the up-pointing magnetic moment is in a top site, which leads to sites with undefined magnetic moments.

# References

[1] K. von Bergmann, M. Menzel, A. Kubetzka, and R. Wiesendanger. Influence of the Local Atom Configuration on a Hexagonal Skyrmion Lattice. *Nano Letters* 15 (2015), 3280–3285.

[2] M. Bode, S. Heinze, A. Kubetzka, O. Pietzsch, X. Nie, G. Bihlmayer, S. Blügel, and R. Wiesendanger. Magnetization-Direction-Dependent Local Electronic Structure Probed by Scanning Tunneling Spectroscopy. *Physical Review Letters* 89 (2002), 237205.
